# Supplementary material for: Animatable Implicit Neural Representations for Creating Realistic Avatars from Videos
Source: arXiv:2203.08133 source file (2023-05-04)

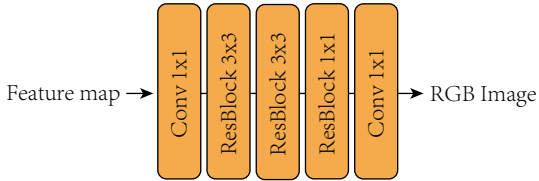

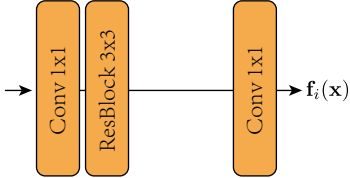

Supplement: Supplementary file 1 [file CNN.pdf]
