# Supplementary material for: Animatable Implicit Neural Representations for Creating Realistic Avatars from Videos
Source: arXiv:2203.08133 source file (2023-05-04)
Supplement: Supplementary file 2 [file 03_supplementary_train_test.tex]

\begin{table}
\begin{center}
\tablestyle{4pt}{1.05}
\begin{tabular}{x{25}|x{15}|x{15}|x{15}|x{15}|x{15}|x{15}|x{15}}
& S1 & S5 & S6 & S7 & S8 & S9 & S11 \\[.1em]
\shline
training & 150 & 250 & 150 & 300 & 250 & 260 & 200 \\
test & 49 & 127 & 83 & 200 & 87 & 133 & 82 \\
\end{tabular}
\end{center}
\caption{\textbf{Frame numbers for training and test of each subject.}}
\vspace{-0.5em}
\label{table:train_test}
\end{table}
